# Supplementary material for: One Model for One Graph: A New Perspective for Pretraining with Cross-domain Graphs
Source: arXiv:2412.00315 source file (2025-05-29)
Supplement: Supplementary file 1 [file contrastive_method.tex]

\section{Results of Other Pretraining Method}

In table~\ref{tab:switch} we attach the results attained by switching self-supervised approaches to GraphMAE. As a comparison, we find that both the original GRACE method and GraphMAE methods could attain similar performance.

\begin{table*}[h]
\centering
%\vspace{-1em}
%\captionsetup{labelfont={color=red}}
\caption{The results for using GraphMAE to pretrain the source models.}
\label{tab:switch}
\resizebox{\linewidth}{!}{
\begin{tabular}{@{}l|lcccccccc@{}}
\toprule
\textbf{Methods} &

 \textbf{Child} &
 \textbf{History} &
\textbf{Cora} &
\textbf{Citeseer} &
\textbf{Dblp} &
\textbf{Products} &
\textbf{Pubmed}&
\textbf{Sports} &
\textbf{Wikics} 
\\ \midrule
\textbf{GraphMAE}  &20.78& 26.51& 64.28& 49.03& 56.88& 31.97& 39.89& 23.65& 61.54      \\
\textbf{Grace} &18.63& 26.39& 63.45& 45.11& 55.11& 30.82& 37.43& 21.73& 60.17     \\ 
\bottomrule
    
\end{tabular}}
\end{table*}
