# Supplementary material for: One Model for One Graph: A New Perspective for Pretraining with Cross-domain Graphs
Source: arXiv:2412.00315 source file (2025-05-29)
Supplement: Supplementary file 2 [file more_baseline_results.tex]

\section{Results of More Baselines}\label{app:more}

We include the results of more baselines of zero-shot node classification and link prediction tasks in table~\ref{tab:baselines}.

\begin{table*}[h]
\centering
%\vspace{-1em}
%\captionsetup{labelfont={color=red}}
\caption{The results for zero-shot learning for more baselines.}
\label{tab:baselines}
\resizebox{\linewidth}{!}{
\begin{tabular}{@{}l|l|lcccccccc@{}}
\toprule
\textbf{Task} &
\textbf{Methods} &

 \textbf{Child} &
 \textbf{History} &
\textbf{Cora} &
\textbf{Citeseer} &
\textbf{Dblp} &
\textbf{Products} &
\textbf{Pubmed}&
\textbf{Sports} &
\textbf{Wikics} 
\\ \midrule
\multirow{4}{*}{\textbf{NC}}& \textbf{GraphMAE}  &15.37& 20.63& 62.83& 46.78& 51.27& 26.23& 33.95& 20.72& 57.98      \\
&\textbf{GCOPE}     &16.83& 20.37& 61.48& 44.26& 53.40& 27.75& 34.26& 19.88& 55.23     \\
&\textbf{GraphAlign} &18.63& 26.39& 63.45& 45.11& 55.11& 30.82& 37.43& 21.73& 60.17     \\ \cmidrule{2-11}
&\textbf{OMOG}      &20.34& 25.68& 66.19& 49.23& 57.53& 31.02& 39.71& 23.65& 62.42  \\ \midrule
\multirow{4}{*}{\textbf{LP}}&\textbf{GraphMAE}  &22.35& 24.15& 51.68& 43.78& 52.28& 33.21& 42.15& 34.20& 49.24      \\
&\textbf{GCOPE}     &24.33& 25.83& 50.24& 44.84& 47.24& 34.85& 45.53& 33.54& 47.29    \\
&\textbf{GraphAlign} &31.81& 32.28& 52.92& 51.34& 51.21& 38.05& 44.28& 35.53& 50.12   \\ \cmidrule{2-11}
&\textbf{OMOG}      &31.29& 34.86& 56.28& 50.72& 53.46& 40.95& 49.42& 37.81& 52.38
    \\ \bottomrule
    
\end{tabular}}
\end{table*}
