# Supplementary material for: One Model for One Graph: A New Perspective for Pretraining with Cross-domain Graphs
Source: arXiv:2412.00315 source file (2025-05-29)
Supplement: Supplementary file 3 [file results.tex]

\section{Numerical Results}\label{app:more2}
We record the numerical values of the ablation study of each dataset in the Table~\ref{tab: ablation}

\begin{table*}[h]
\centering
%\vspace{-1em}
\caption{The results for zero-shot node classification.}
\label{tab: ablation}
\resizebox{\linewidth}{!}{
\begin{tabular}{@{}l|l|lcccccccc@{}}
\toprule
\textbf{Task} &
\textbf{Methods} &

 \textbf{Child} &
 \textbf{History} &
\textbf{Cora} &
\textbf{Citeseer} &
\textbf{Dblp} &
\textbf{Products} &
\textbf{Pubmed}&
\textbf{Sports} &
 \textbf{Wikics} 
\\ \midrule
\multirow{4}{*}{\textbf{NC}}& \textbf{No SGC}               
                                  & 17.23 & 23.91 & 61.73 & 47.82 & 52.74 & 29.56 & 37.62 & 20.47 & 60.35      \\
&\textbf{No Score}                 & 16.03 & 23.29 & 60.84 & 45.11 & 53.98 & 27.17 & 34.76 & 18.12 & 58.72     \\
&\textbf{No Source}               & 18.83 & 23.42 & 64.43 & 46.93 & 53.89 & 28.63 & 36.22 & 19.47 & 59.73     \\ \cmidrule{2-11}
&\textbf{OMOG}                     & 20.34 & 25.68 & 66.19 & 49.23 & 57.53 & 31.02 & 39.71 & 23.65 & 62.42  
    \\ \midrule
\multirow{4}{*}{\textbf{LP}}&\textbf{No SGC}              
                                 & 28.63 & 31.30 & 54.18 & 49.57 & 49.76 & 37.43 & 45.84 & 34.92 & 47.26      \\
&\textbf{No Score}                 & 29.11 & 32.61 & 54.84 & 48.63 & 48.40 & 38.57 & 46.62 & 35.86 & 51.28     \\
&\textbf{No Source}              & 29.75 & 33.92 & 55.28 & 49.71 & 50.08 & 37.93 & 47.38 & 35.94 & 50.48   \\ \cmidrule{2-11}
&\textbf{OMOG}                & 31.29 & 34.86 & 56.28 & 50.72 & 53.46 & 40.95 & 49.42 & 37.81 & 52.38 
    \\ \bottomrule
    
\end{tabular}}
\end{table*}
